# Supplementary material for: VidHarm: A Clip Based Dataset for Harmful Content Detection
Source: arXiv:2106.08323 source file (2022-09-02)
Supplement: Supplementary file 1 [file supplementary.tex]

\section{Qualitative Results}
\subsection{Qualitative Results}
Here we show challenging clips from the dataset and the corresponding predictions from the trained models. We additionally showcase a failure case as well as a clip where it is unclear if an objective way to label exists. To compare predictions we selected a single trained model for both modalities. We additionally provide the fused predictions.

\parsection{Example 1}
In this clip (see \url{https://youtu.be/8LQAPED-7zA}) from the trailer of \emph{The Deep} (2012), a boat has capsized with crew members trying not to drown. Both models manage to predict the 11+ rating.
\begin{figure}[h!]
\includegraphics[width=\linewidth]{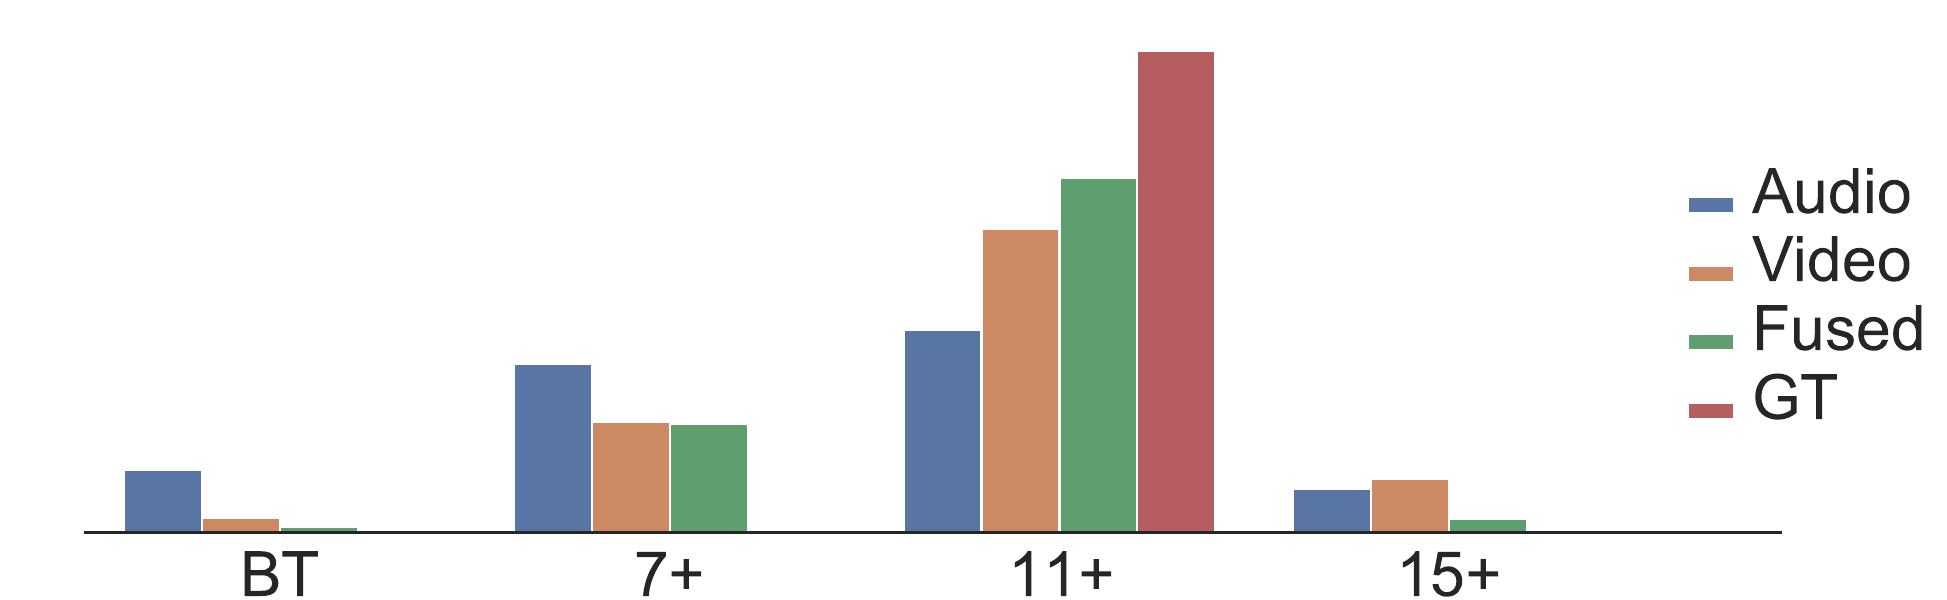}
    \caption{Predictions for Example 1.}
    \label{fig:my_label}
\end{figure}

\parsection{Example 2}
In this clip (see \url{https://youtu.be/GrMXRRxrGeI}) from the trailer of \emph{Discarnate} (2018), the monster of the movie is introduced. The audio is frightening and the visual content is disturbing. Both modalities accurately predict the rating to be between 11+/15+.
\begin{figure}[h!]
\includegraphics[width=\linewidth]{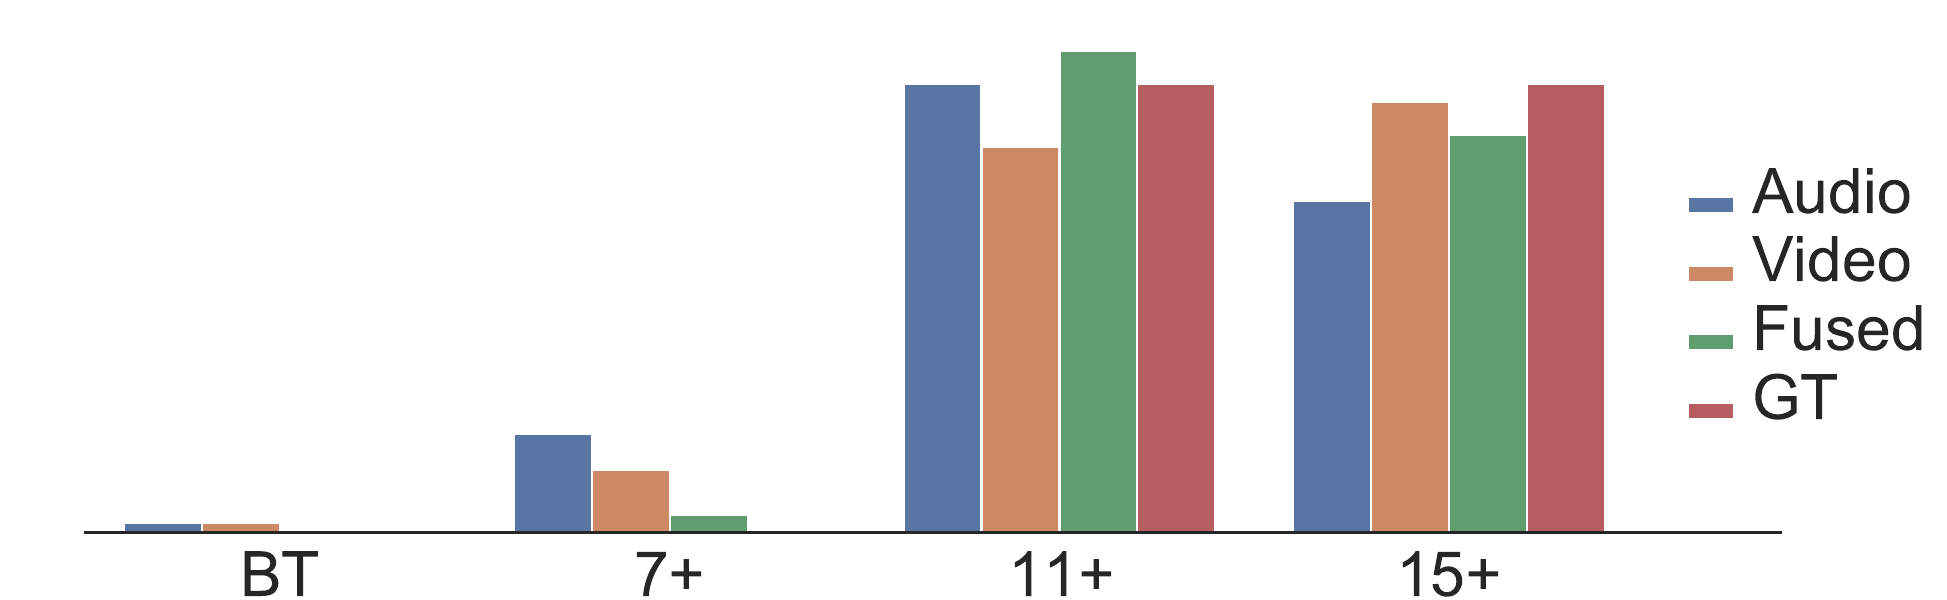}
    \caption{Predictions for Example 2.}
    \label{fig:my_label}
\end{figure}

\parsection{Example 3}
In this very challenging scene (see \url{https://youtu.be/4-sAYL67y3M}) from the trailer of \emph{A Second Chance} (2014), no direct violence or horror is present. However, there is a tense mood and the scene could perhaps be considered to contain harmful content. While the human labels annotate the scene as BT, the models indicate an inherent uncertainty in the harmfulness.
\begin{figure}[h!]
    \includegraphics[width=\linewidth]{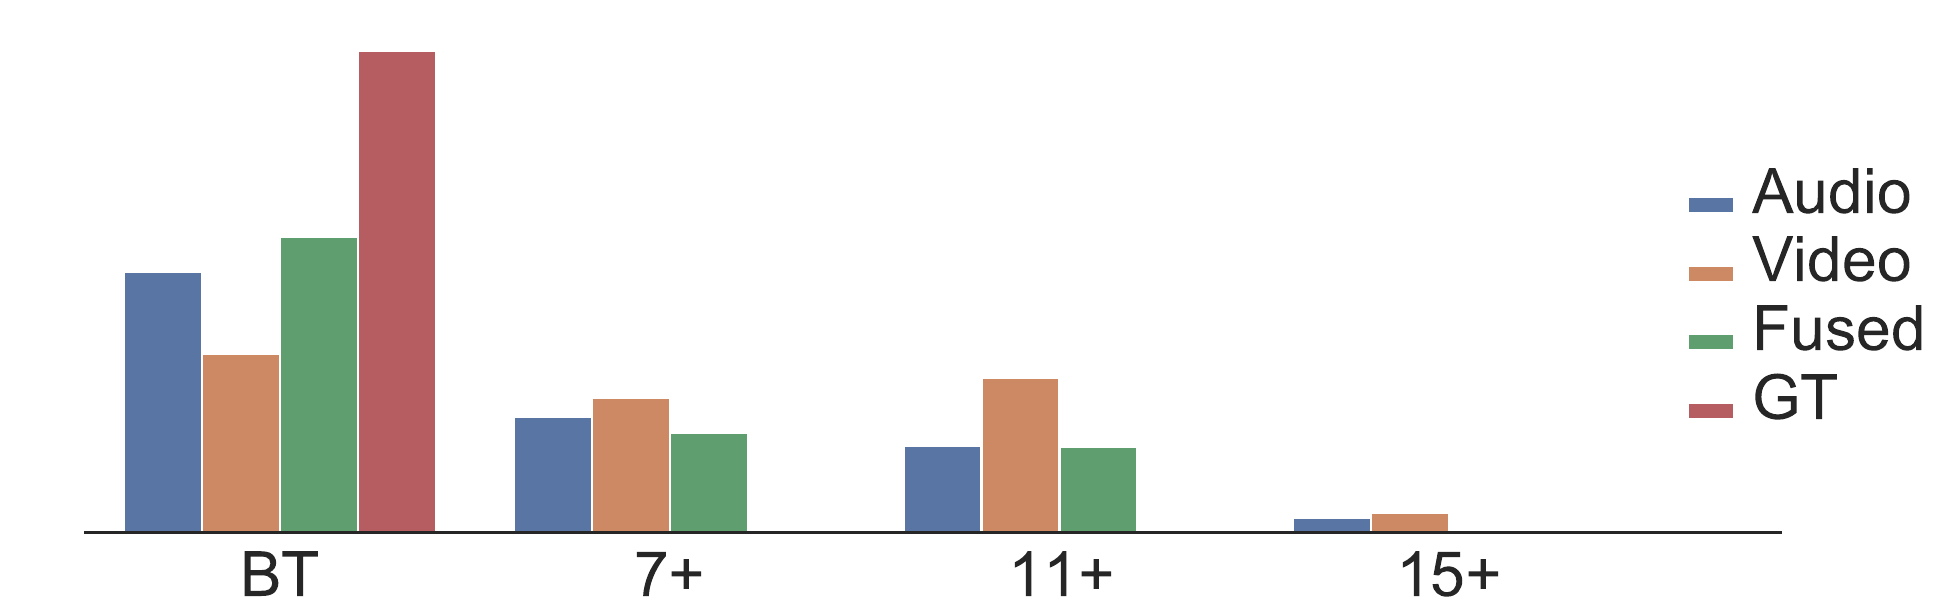}
    \caption{Predictions for Example 3.}
    \label{fig:my_label}
\end{figure}

\parsection{Example 4}
Here we show a rare failure case. In this scene (see \url{https://youtu.be/FwavMLSOtv4}) from the trailer of \emph{City State} (2011), a naked man is threatened with a rifle. However, both the visual and audio models underestimate the harmful content in this clip.
\begin{figure}[h!]
\includegraphics[width=\linewidth]{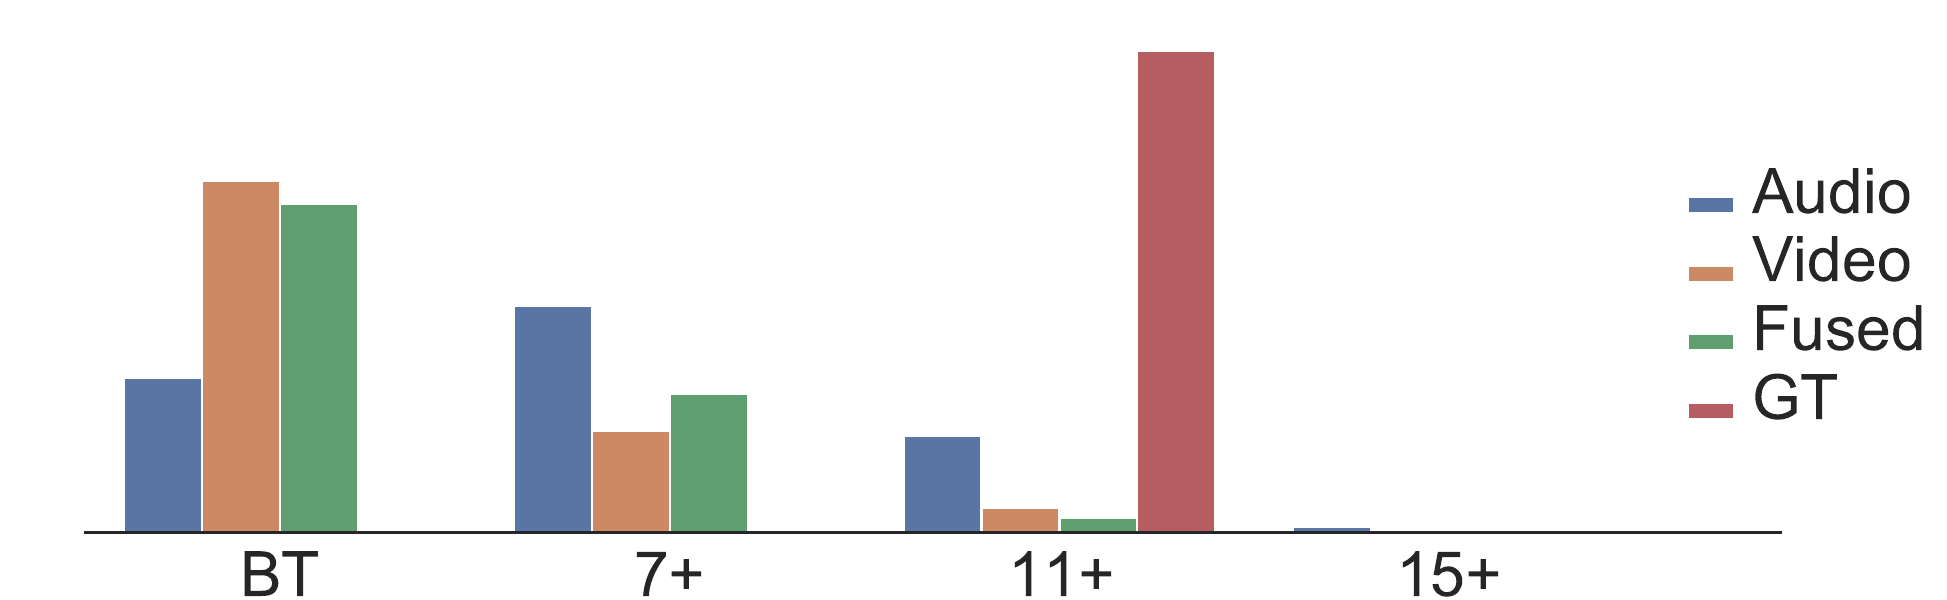}
    \caption{Predictions for Example 4.}
    \label{fig:my_label}
\end{figure}

\subsection{Modality Matters}
An interesting topic is that of evaluating what kinds of harmful content can be detected from the visual modality but not the audio modality and vice versa. Here we show a set of qualitative examples where one modality can correctly estimate the harmfulness, but not the other.

\parsection{Example 5}
In this scene (see \url{https://youtu.be/UQki0nl-ukc}) from the trailer of \emph{Paydirt} (2020) intense music can be heard and firearms are discussed. However, the scene is humorous and the content is not harmful. The video model correctly estimates the rating to be BT, while the audio model is uncertain and spreads out its predictions, likely due to the intense soundtrack at the start of the clip.
\begin{figure}[h!]

\includegraphics[width=\linewidth]{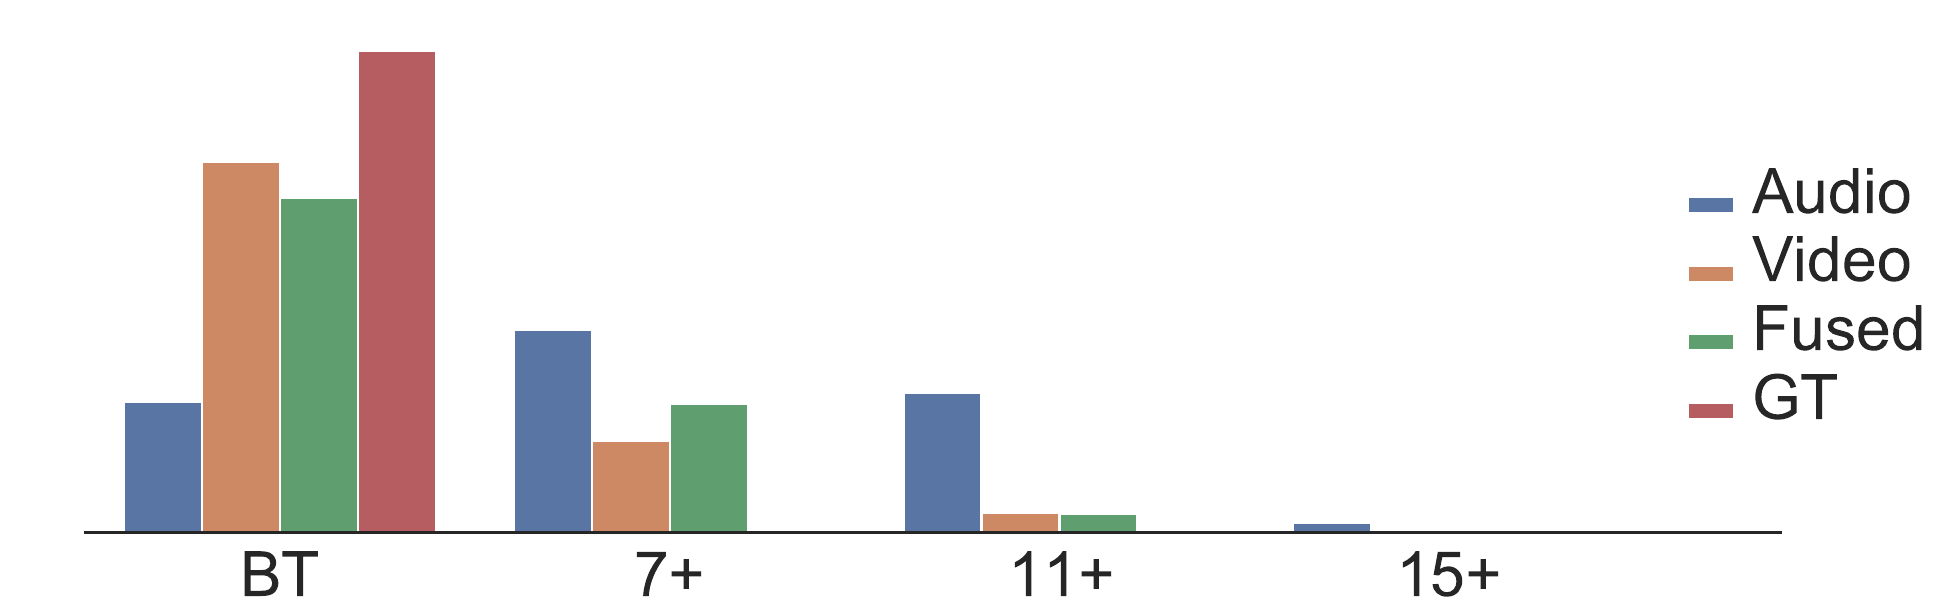}
    \caption{Predictions for Example 5.}
    \label{fig:my_label}
\end{figure}

\parsection{Example 6}
In this example (see \url{https://youtu.be/_ZR13_U4VPA}) from the trailer of \emph{For Sama} (2019) the musical score is melancholic and slightly threatening, but the visual content is not threatening. The visual model correctly identifies the label, while the audio model gives an uncertain estimate.
\begin{figure}[h!]
    \includegraphics[width=\linewidth]{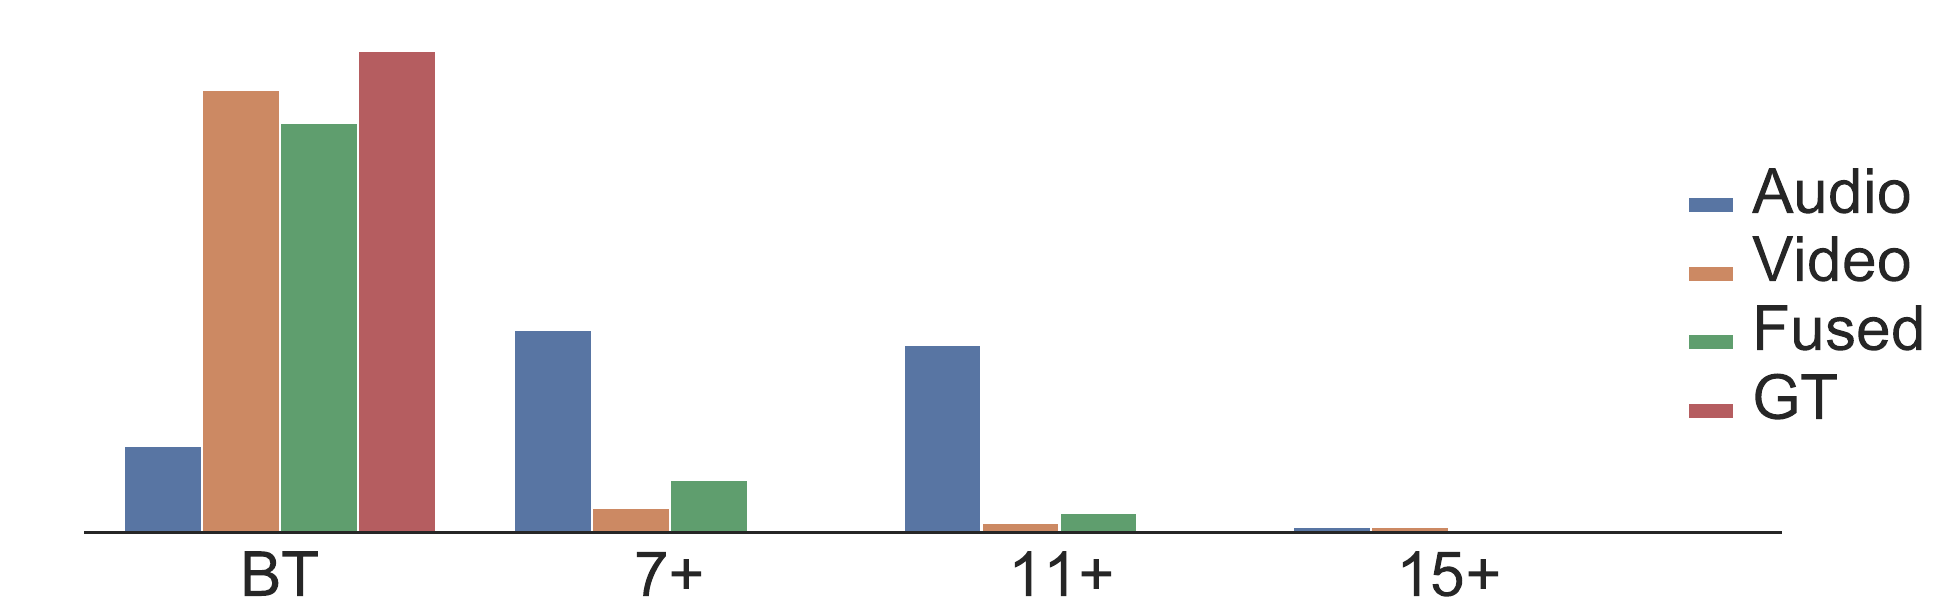}
    \caption{Predictions for Example 6.}
    \label{fig:my_label}
\end{figure}

\parsection{Example 7}
In this clip (see \url{https://youtu.be/GdhYe4E5iWY}) from the trailer of \emph{Virgin Mountain} (2015), there are multiple threatening visual cues with, e.g., a window being broken. However, the music de-dramatizes the clip and has hence received a BT rating. This is accurately conveyed in the predictions from the corresponding modalities.
\begin{figure}[h!]
\includegraphics[width=\linewidth]{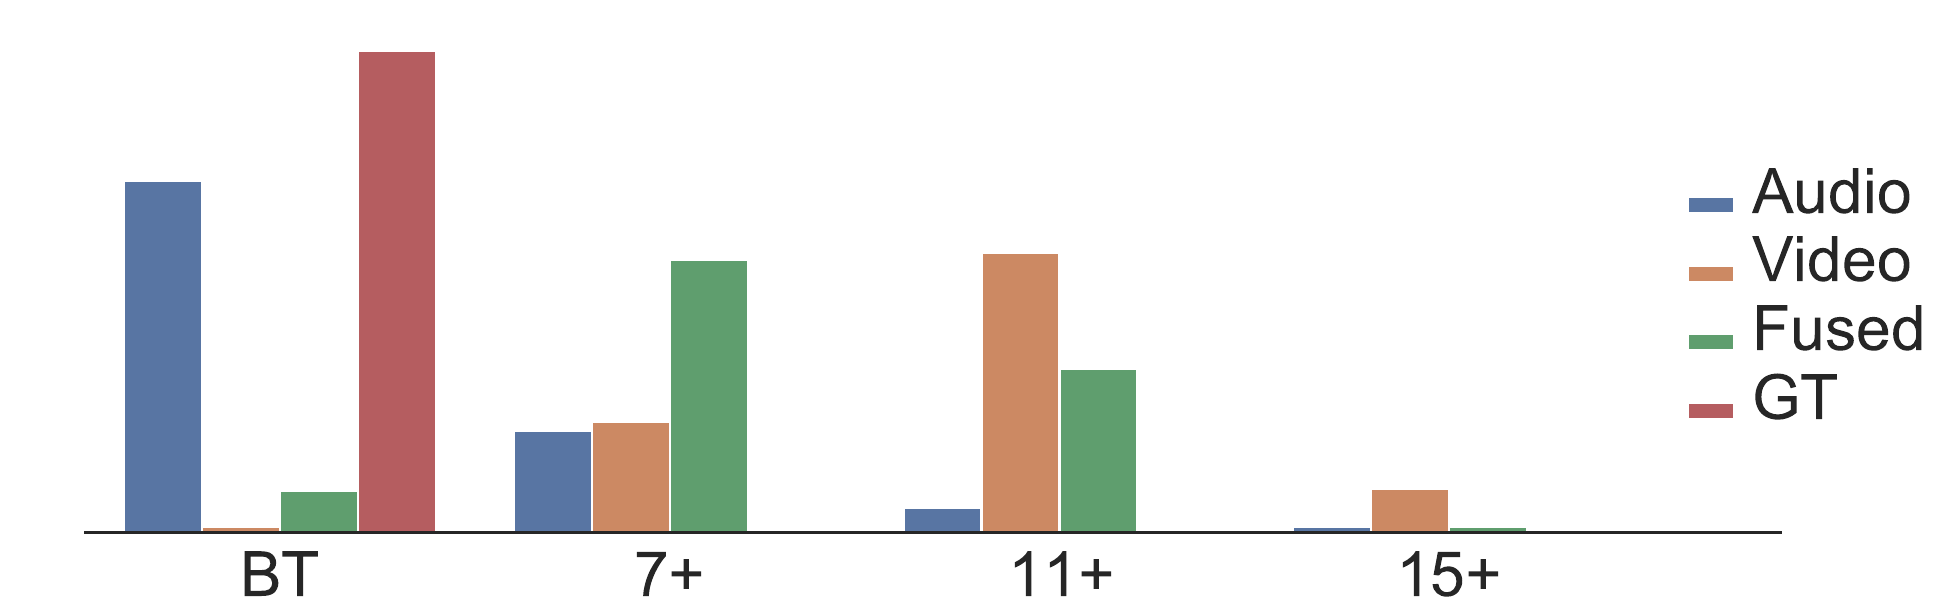}
    \caption{Predictions for Example 7.}
    \label{fig:my_label}
\end{figure}

Here we will provide some additional qualitative examples with corresponding predictions on our dataset.

\parsection{Example S-1}
In this clip (see \url{https://youtu.be/6OQfccBu3Qo}) from the trailer of \emph{Aus dem Nichts} (2017), a woman is greatly distressed, and death is implied. Both predictions from both modalities closely match the ground truth ratings.
\begin{figure}[h!]
\includegraphics[width=\linewidth]{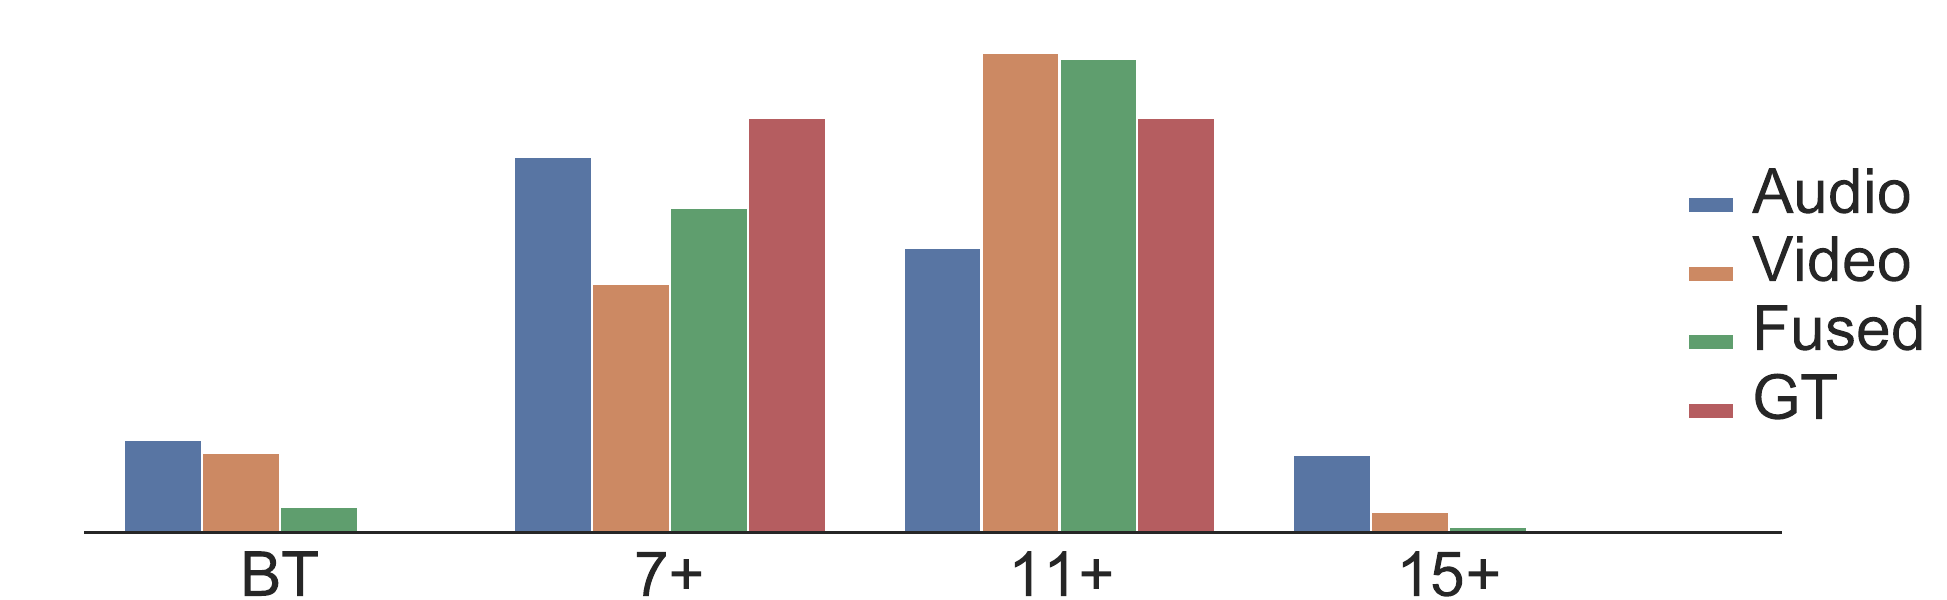}
    \caption{Predictions for Example S-1.}
    \label{fig:my_label}
\end{figure}

\parsection{Example S-2}
In this clip (see \url{https://youtu.be/NUCiKTcWF94}) from the trailer of \emph{A Season in France} (2017) a father is discussing having to move with his children. Both modalities give accurate predictions.
\begin{figure}[h!]
\includegraphics[width=\linewidth]{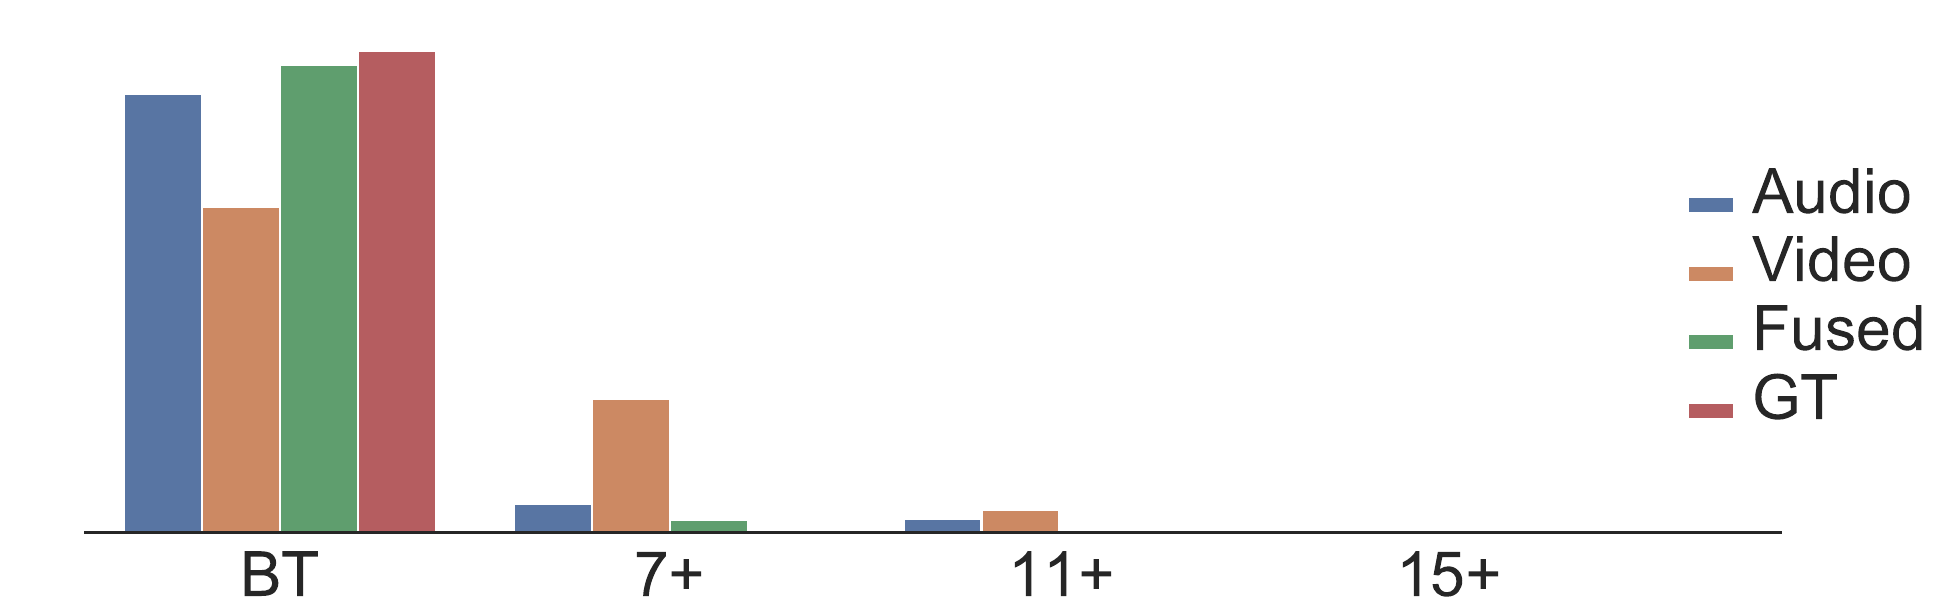}
    \caption{Predictions for Example S-2.}
    \label{fig:my_label}
\end{figure}

\parsection{Example S-3}
In this clip (see \url{https://youtu.be/T3DEWyloZJs}) from the trailer of \emph{Beauty and the Dogs} (2017), a woman is escaping several men in a corridor. Both modalities slightly underestimate the harmfulness, perhaps underestimating the context.
\begin{figure}[h!]
\includegraphics[width=\linewidth]{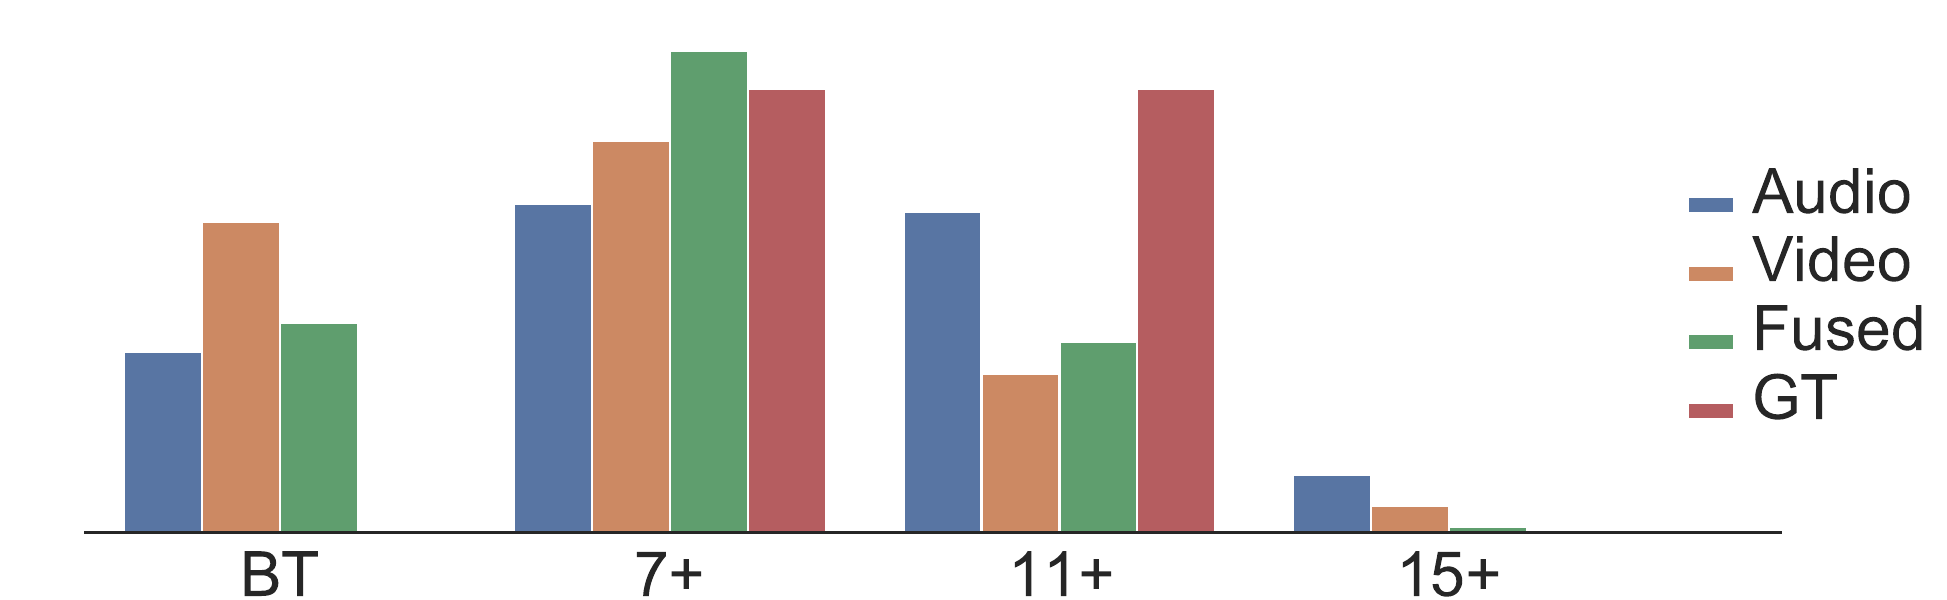}
    \caption{Predictions for Example S-3.}
    \label{fig:my_label}
\end{figure}

\parsection{Example S-4}
This clip (see \url{https://youtu.be/YwiRV3Dmugs}) from the trailer of \emph{The Silent Revolution} (2018) contains harsh language and violence, and has a threatening context. Both modalities correctly identify the 7+ rating.
\begin{figure}[h!]
\includegraphics[width=\linewidth]{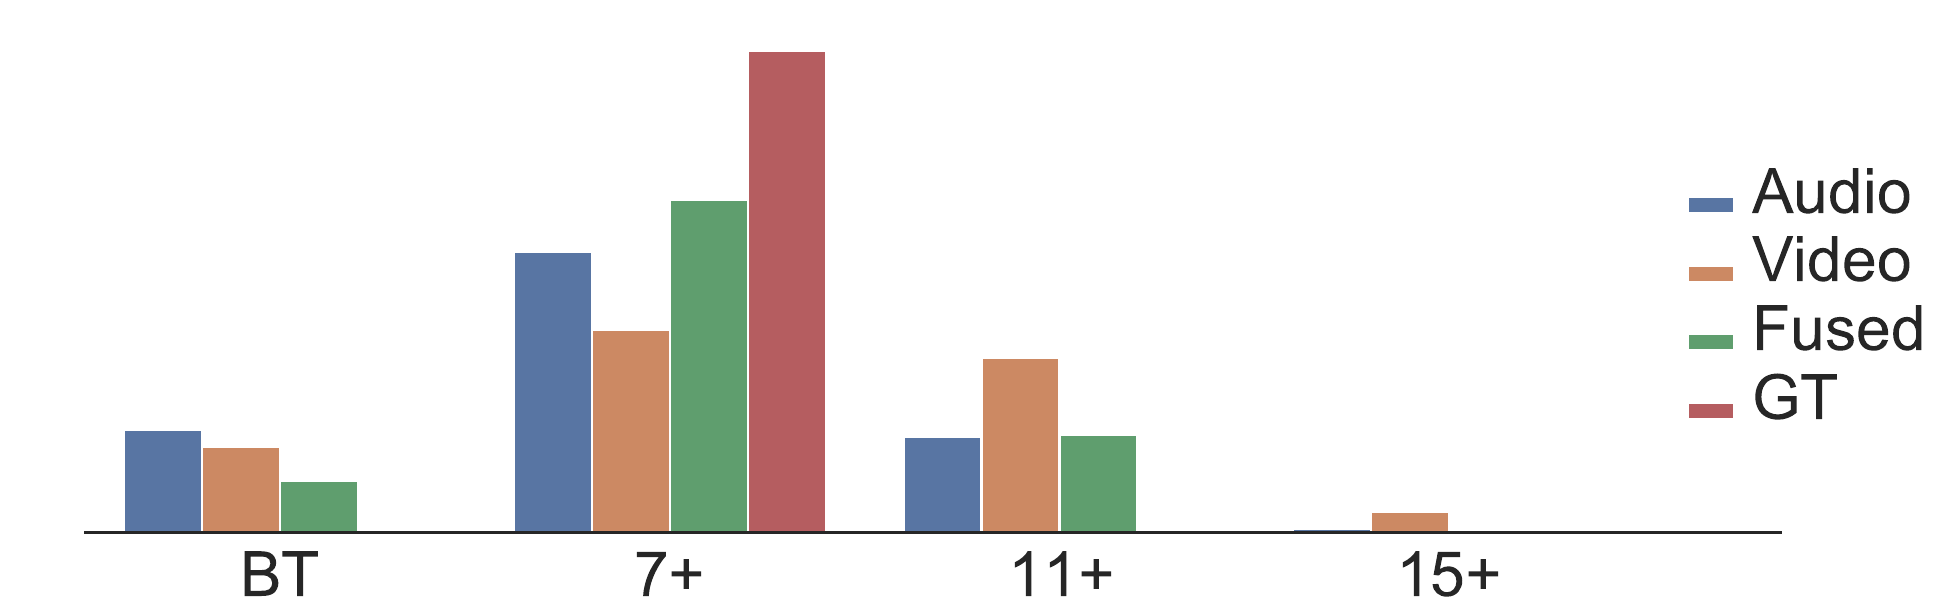}
    \caption{Predictions for Example S-4.}
    \label{fig:my_label}
\end{figure}

\parsection{Example S-5}
In this clip (see \url{https://youtu.be/bOOE_NeUwqc}) from the trailer of \emph{BPM (Beats Per Minute)} (2017), a multitude of dramatic scenes are shown in rapid succession. The audio is, however, not particularly threatening. Here the prediction from the visual model clearly fails, while the audio model performs better.
\begin{figure}[h!]
\includegraphics[width=\linewidth]{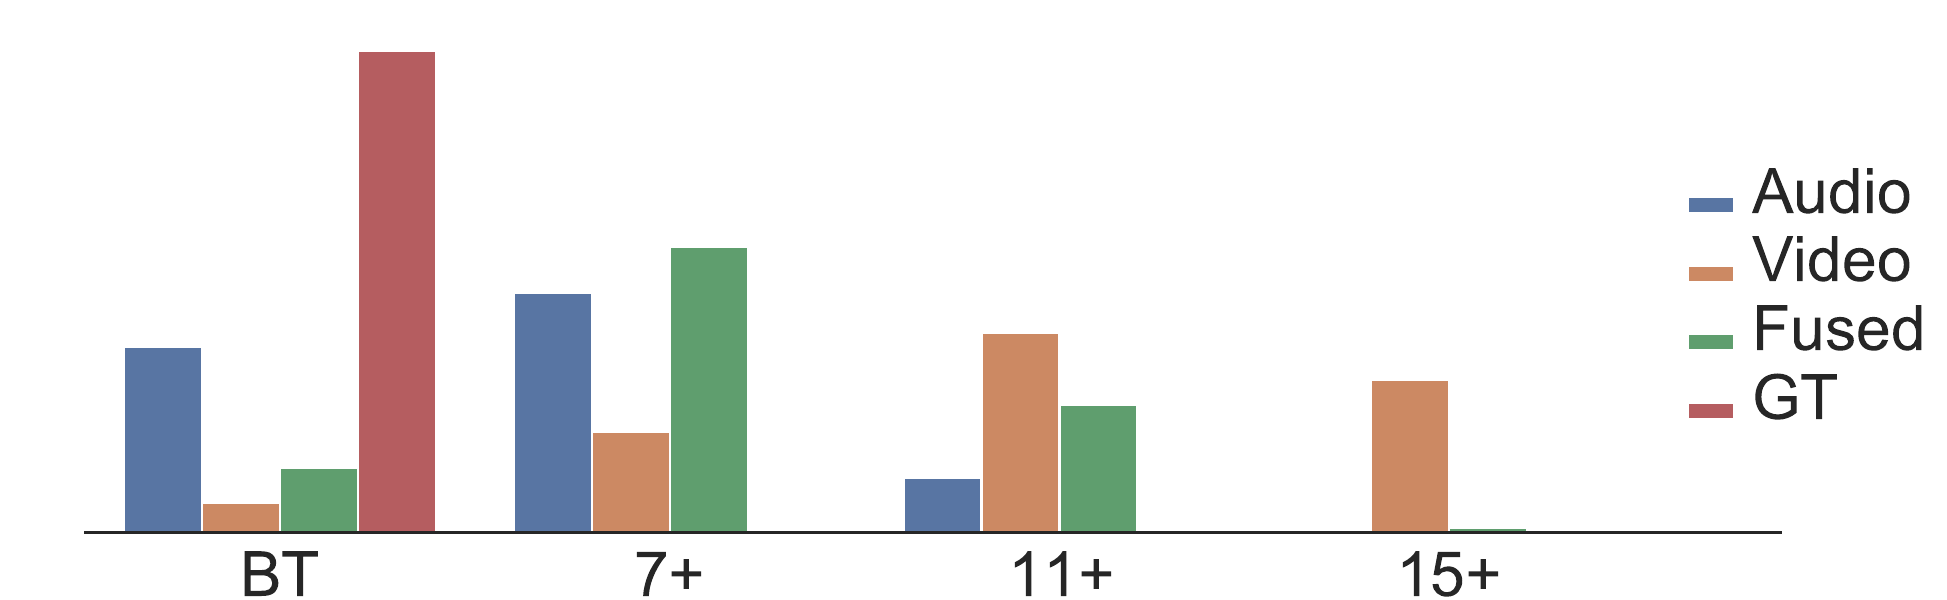}
    \caption{Predictions for Example S-5.}
    \label{fig:my_label}
\end{figure}

\parsection{Example S-6}
In this clip (see \url{https://youtu.be/HG9G0rrvnCI}) from the trailer of \emph{The Kidnapping of Michel Houellebecq} (2014), a somewhat loud discussion is taking place, with a telephone ringing in the background. Predictions from both modalities correctly identify the clip to not contain any harmful content.
\begin{figure}[h!]
\includegraphics[width=\linewidth]{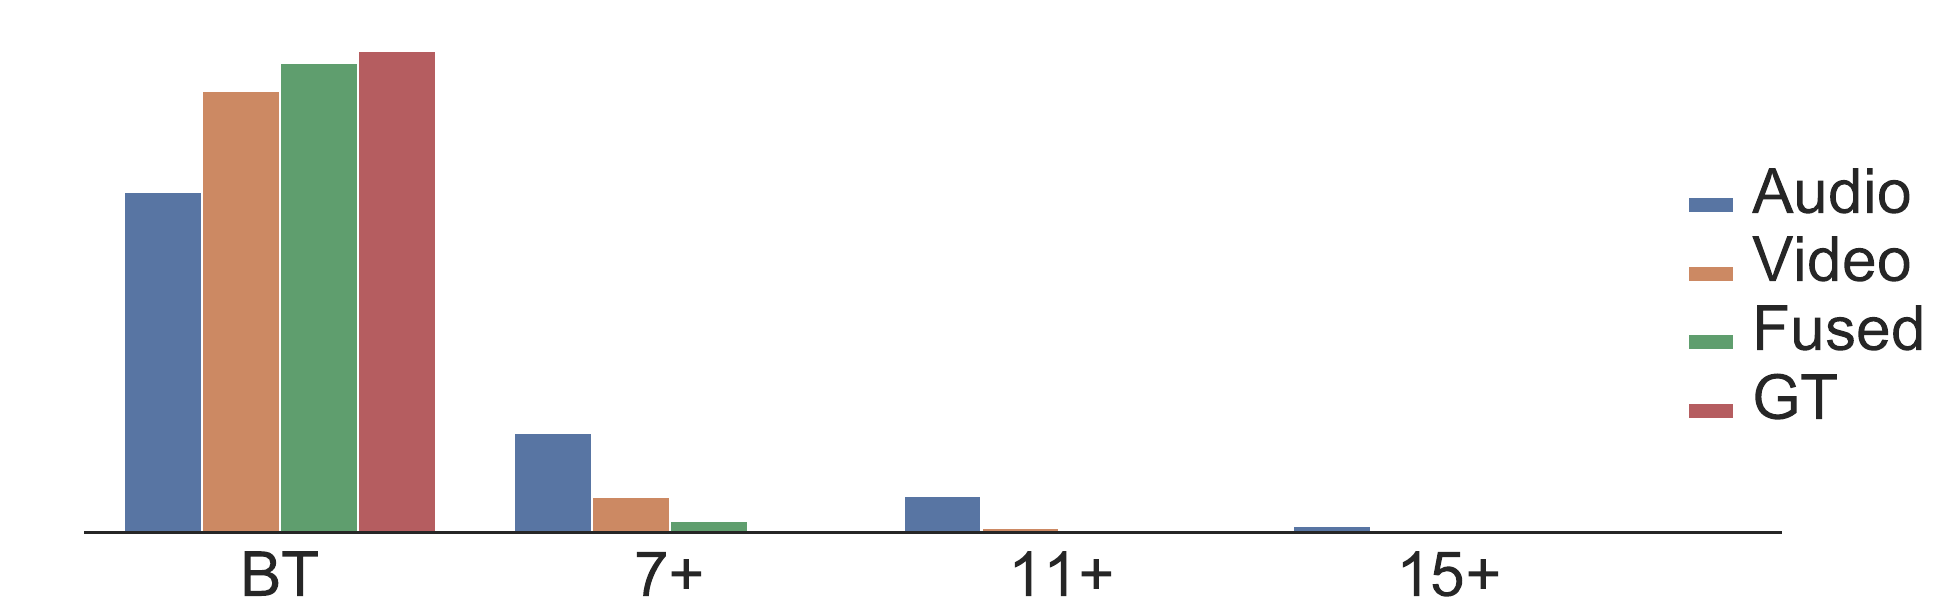}
    \caption{Predictions for Example S-6.}
    \label{fig:my_label}
\end{figure}

%\parsection{Example S-7}
%In this clip (see \url{https://youtu.be/2sl-lhL6o5g}) from the trailer of \emph{x} (y),.
%\begin{figure}[h!]
%\includegraphics[width=\linewidth]{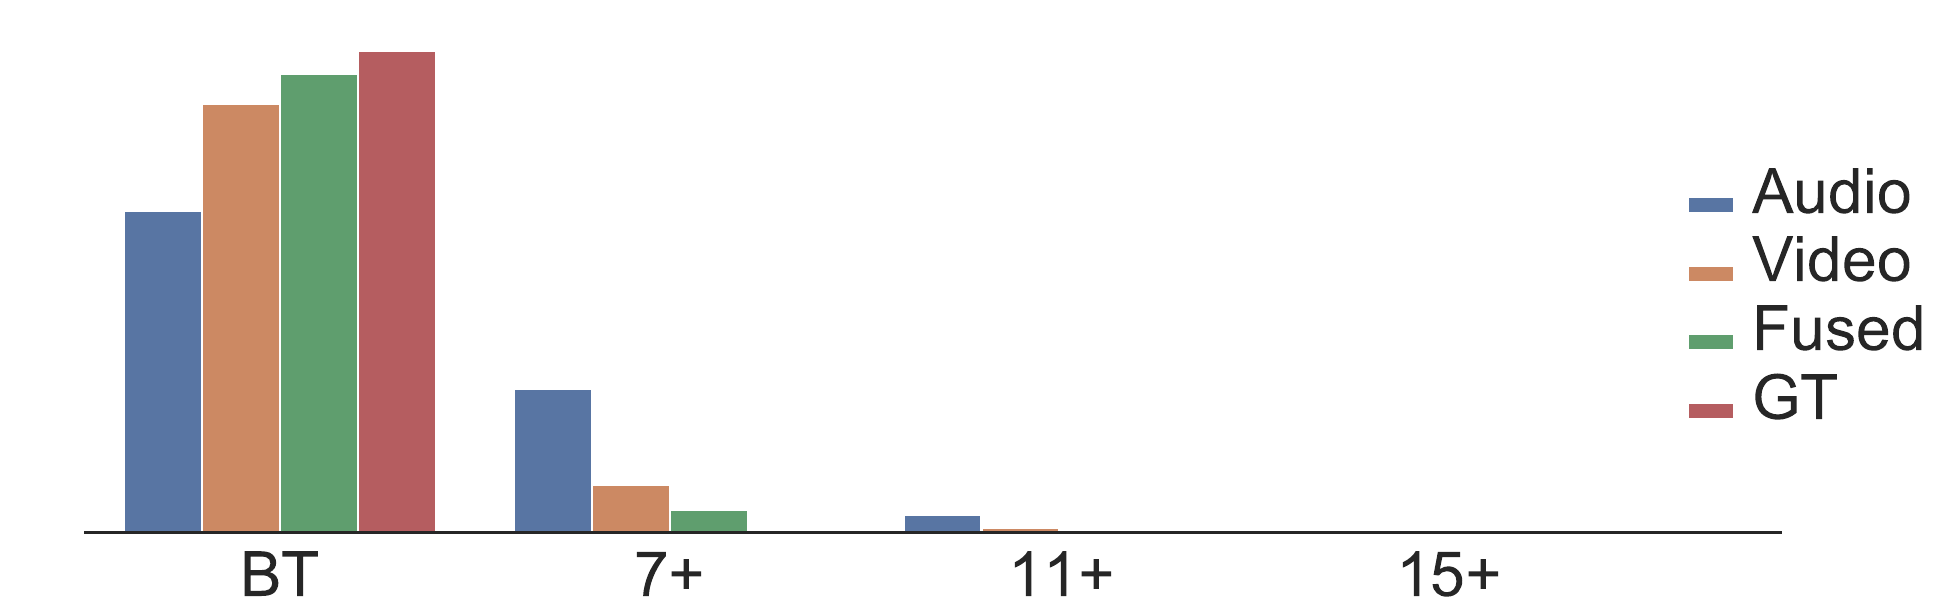}
%    \caption{Predictions for Example S-7.}
%    \label{fig:my_label}
%\end{figure}

%\parsection{Example S-7}
%In this clip (see \url{https://youtu.be/5WKnxyU_lQY}) from the trailer of \emph{x} (y),.
%\begin{figure}[h!]
%\includegraphics[width=\linewidth]{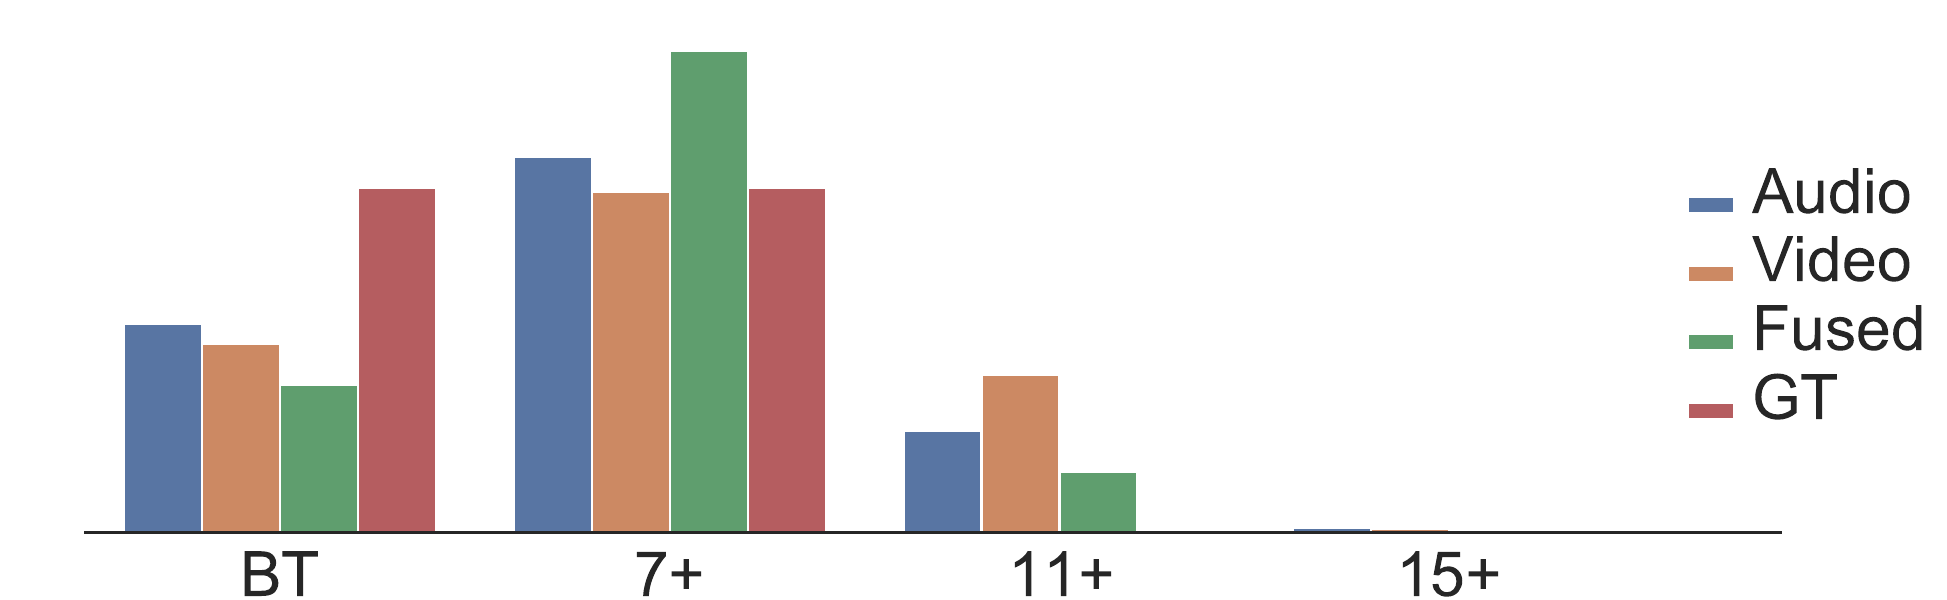}
%    \caption{Predictions for Example S-7.}
%    \label{fig:my_label}
%\end{figure}
